# Supplementary material for: CANDY: A Benchmark for Continuous Approximate Nearest Neighbor Search with Dynamic Data Ingestion
Source: arXiv:2406.19651 source file (2024-06-28)
Supplement: Supplementary file 1 [file OptAppendix.tex]

\textbf{Machine Learning Leads to Large Improvements, But Challenged by Distribution Shifts.}
\begin{table}[]
\resizebox{0.99\textwidth}{!}{%

\begin{tabular}{|l|l|l|l|l|l|}
\hline
Case                                 & Algoroithms & Recall@10 & Query Latency & Vector Search Latency & Pending Write Latency \\ \hline
\multirow{3}{*}{No Shift} & \algoBF     & 1.000     & 0.19          & 0.12                  & 0.07                  \\ \cline{2-6} 
                                     & AKNN w/o ML & 0.003     & 0.03          & 0.01                  & 0.03                  \\ \cline{2-6} 
                                     & AKNN w/ ML  & 0.024     & 0.10          & 0.10                  & 0.01                  \\ \hline
\multirow{3}{*}{Use Shift}  & \algoBF     & 1.000     & 0.21          & 0.14                  & 0.07                  \\ \cline{2-6} 
                                     & AKNN w/o ML & 0.003     & 0.04          & 0.01                  & 0.03                  \\ \cline{2-6} 
                                     & AKNN w/ ML  & 0.374     & 5.82          & 5.82                  & 0.01                  \\ \hline
\end{tabular}
}
\caption{AKNN with machine learning. The unit of latency is $\times 1000ms$.}
\label{tab:opt_aknn_ml}
\end{table}
We select the \algoLSH as the example to study the impact of using matching learning.
For a fair comparison, we optimize \algoLSH by replacing its random projection hash function with a pre-trained neural networks, while keeping other data structures and workflows the same. As demonstrated in Table~\ref{tab:opt_aknn_ml}, using machine learning significantly improves the accuracy by at least $ 7\times$.
The query latency and vector search latency are increased when using machine learning, and they are mostly caused by the static overhead of using neural networks. However, they are still attractive compared with \algoBF, i.e., $45\%$ less query latency.  
Furthermore, we observe that machine learning reduces the pending writing latency of AKNN (i.e., $66\%$ less compared with raw \algoLSH), as it
leads to a more accurate assignment of interested vectors.

Nevertheless, how to handle the distribution shifts is still an opening challenge for machine learning itself, and the suboptimal performance of learning leads to a significant performance downgrade of AKNN. 
Although the recall seems to be even better, i.e., $0.374$ in this case, the query latency is extremely high. This is because the AKNN can not find the straight-forward matches under ML-based \algoLSH during the distribution shift, therefore, it downgrades into an exhaustive traverse on all of the buckets, which is even more costly than \algoBF.
We envision more advanced techniques such as online continual learning~\cite{li2022camel} to solve this problem, as well as solving other related implementation issues like re-encoding the existing buckets~\cite{xu2018online}. 

\textbf{Optimized Distance Computation is also Helpful, but the Ingestion Efficiency Challenge is Still Pressing.}
We selected \algoHNSW as our example to examine the impacts of optimized distance computation. We adhered to the methodologies outlined in \cite{aguerrebere2024locally} for data compression and in \cite{gao2023high} for randomized computation. The results of these optimizations are displayed in Table~\ref{tab:opt_aknn_dis}.
Overall, both optimizations proved beneficial in reducing the AKNN overhead associated with writing and searching, therefore decreasing overall query latency—by up to $81.7\%$ in scenarios utilizing compression.
As anticipated, these gains in efficiency come at the cost of a slight reduction in query recall.
Nonetheless, the challenge of ingestion efficiency remains critical, as even optimized AKNN systems do not surpass \algoBF in query latency due to the substantial overhead still associated with pending writes.
Moreover, we observed that poor ingestion efficiency diminishes the resilience of AKNN optimizations to data distribution shifts. For instance, the recall dropped to 0.09 with compression compared to 0.48 for the original AKNN setup. Although the compression optimization outlined in \cite{aguerrebere2024locally} aims to mitigate distribution shifts, its effectiveness depends on continuous observation of ingested data.
If substantial data is dropped due to ingestion inefficiencies, these observations become biased, leading to the failure of this countermeasure.
We recognize that variational inference ~\cite{zeng2024pecj, alsaedi2023radar, bai2020efficient, rudner2022tractable} may offer a solution to correct these biased observations. However, integrating it into AKNN optimizations presents a novel challenge that warrants further investigation.

\xianzhi{--@ zhuoyan @xinjing xxxx}
 For data compression, our optimization employs Locally-Adaptive Vector Quantization (LVQ). LVQ involves maintaining a global mean vector and performing scalar quantization on input vectors using this mean vector along with local maximum and minimum values. This process encodes data into short integers, which are used for distance computation during search, effectively reducing cost.
 For randomized computation, our optimization employs ADSampling. ADSampling involves randomly transforming the input and query vectors with a transform matrix, and distances will be calculated between transformed vectors in a stepwise manner, i.e., intermediate distance values be compared against a threshold in each step. The distance computation will be eliminated in advance if the intermediate distance value is greater than the threshold, and the threshold is a proportion of the largest value in the results heap.

\begin{table}[]
\resizebox{0.99\textwidth}{!}{%
\begin{tabular}{|l|l|l|l|l|l|}
\hline
Case                                 & Algoroithms   & Recall@10 & Query Latency & Vector Search Latency & Pending Write Latency \\ \hline
\multirow{4}{*}{No Shift} & \algoBF       & 1.00      & 0.19          & 0.12                  & 0.07                  \\ \cline{2-6} 
                                     & AKNN          & 0.41      & 485.53        & 47.78                 & 437.75                \\ \cline{2-6} 
                                     & AKNN w/ comp. & 0.30      & 99.32         & 0.08                  & 99.24                 \\ \cline{2-6} 
                                     & AKNN w/ rand. & 0.00      & 89.01         & 0.08                  & 88.94                 \\ \hline
\multirow{4}{*}{Use Shift}  & \algoBF       & 1.00      & 0.21          & 0.14                  & 0.07                  \\ \cline{2-6} 
                                     & AKNN          & 0.48      & 20.15         & 0.08                  & 0.03                  \\ \cline{2-6} 
                                     & AKNN w/ comp. & 0.09      & 15.41         & 0.07                  & 15.34                 \\ \cline{2-6} 
                                     & AKNN w/ rand. & 0.01      & 12.90         & 0.07                  & 12.83                 \\ \hline
\end{tabular}
}
\caption{AKNN with optimized distance computation. The unit of latency is $\times 1000ms$. `Comp.' is short for compression~\cite{aguerrebere2024locally}, and `rand.' is short for randomized calculation~\cite{gao2023high}, }
\label{tab:opt_aknn_dis}
\end{table}
